# Supplementary material for: Finding Backdoors to Integer Programs: A Monte Carlo Tree Search Framework
Source: arXiv:2110.08423 source file (2022-07-07)
Supplement: Supplementary file 1 [file appendix.tex]

% \section{Missing sentence in ``Algorithm Engineering"}
% The last sentence of paragraph ``Algorithm Engineering" on page 5 of the main text was accidentally left incomplete; we correct it here:

% \textit{Rather than simulate and evaluate a single candidate at a time, we leverage the independence between the simulations to execute them and the candidate evaluation in parallel.}

\section{Further definitions}
\label{appendix:definitions}

\subsection{Shifted Geometric Means in Table~\ref{tab:mipresults}}

Compared to arithmetic means, geometric means are more robust to measurements that are extremely small or large. That is why they are the standard method for aggregating both the number of (branch-and-bound) nodes and total running time in MIP solving. The \textit{shifts} are used to eliminate large \textit{relative variations} between two methods, even when in absolute terms these variations are likely insignificant, e.g., for the same instance, two solvers A and B record running times of 0.8 and 1 second which suggests a substantial 20\% improvement for A over B, whereas wall-clock times can exhibit similar fluctuations for reasons not related to the actual solvers themselves. We refer to page 33 of~\citep{Hendel15} for further discussion. 

The shifted geometric mean with shift $\tau$ for a set of measurements $(X_i)_{i=1}^q$ is:
$$\bar{X}^\tau=\Bigg( \prod_{i=1}^q (X_i + \tau)\Bigg)^{\frac{1}{q}} - \tau.$$
We use the standard shifts of $\tau=10$ seconds for total time and $\tau=100$ nodes for total nodes.

\section{Additional Experimental Results}

\subsection{Full \bamcts~Hyperparameter Tuning Results}

\begin{table}[hb]
\centering
\small
\resizebox{\columnwidth}{!}{%
\begin{tabular}{@{}ccccccc@{}}
\toprule
  \multicolumn{1}{l}{} &
  \multicolumn{1}{l}{Backup} &
  \begin{tabular}[c]{@{}c@{}}Exp. \\ Type\end{tabular} &
  \begin{tabular}[c]{@{}c@{}}\texttt{use\_}\\\texttt{variance}\end{tabular} &
  $\alpha_{\text{PC}}$ & 
  $C$ &
  \begin{tabular}[c]{@{}c@{}}Mean\\ Reward\end{tabular} \\ \midrule
\textbf{10}    &   max &   Uniform &  False &    0.00 &    $\sqrt{2}$   &  0.208 \\
\textbf{23}    &   sum &   Uniform &  False &    0.50 &    $1/\sqrt{2}$ &  0.286 \\
\textbf{22}    &   max &   Uniform &  False &    0.00 &    $2$          &  0.289 \\
\textbf{20}    &   sum &   Uniform &  True  &    0.10 &    $2$          &  0.291 \\
\textbf{11}    &   max &   Uniform &  True  &    0.00 &    $2$          &  0.293 \\
\textbf{19}    &   max &   Uniform &  False &    0.01 &    $1/\sqrt{2}$ &  0.295 \\
\textbf{21}    &   sum &   Uniform &  False &    0.00 &    $\sqrt{2}$   &  0.297 \\
\textbf{16}    &   sum &   Uniform &  False &    0.50 &    $\sqrt{3}$   &  0.304 \\
\textbf{12}    &   max &   Uniform &  True  &    0.50 &    $2$          &  0.304 \\
\textbf{7}     &   max &   Uniform &  True  &    0.00 &    $\sqrt{3}$   &  0.306 \\
\textbf{3}     &   max &   Uniform &  False &    0.01 &    $\sqrt{3}$   &  0.307 \\
\textbf{9}     &   max &   Uniform &  True  &    0.10 &    $2$          &  0.313 \\
\textbf{0}     &   sum &   Uniform &  False &    0.01 &    $2$          &  0.313 \\
\textbf{17}    &   sum &   Uniform &  False &    0.50 &    $1$          &  0.315 \\
\textbf{6}     &   sum &   Uniform &  True  &    0.00 &    $\sqrt{2}$   &  0.315 \\
\textbf{26}    &   max &   Uniform &  True  &    0.01 &    $1/\sqrt{2}$ &  0.320 \\
\textbf{2}     &   max &   Uniform &  True  &    0.00 &    $1/\sqrt{2}$ &  0.322 \\
\textbf{4}     &   sum &   Best    &  False &    0.00 &    $2$          &  0.327 \\
\textbf{25}    &   max &   Best    &  False &    0.01 &    $1$          &  0.330 \\
\textbf{15}    &   max &   Best    &  True  &    0.50 &    $2$          &  0.332 \\
\textbf{5}     &   max &   Best    &  False &    0.01 &    $\sqrt{3}$   &  0.333 \\
\textbf{8}     &   sum &   Best    &  False &    0.01 &    $\sqrt{3}$   &  0.337 \\
\textbf{1}     &   max &   Best    &  False &    0.50 &    $\sqrt{2}$   &  0.337 \\
\textbf{13}    &   max &   Best    &  False &    0.10 &    $1$          &  0.343 \\
\textbf{24}    &   max &   Best    &  True  &    0.01 &    $1$          &  0.351 \\
\bottomrule
\end{tabular}}
\caption{\small All \bamcts~parameter configurations sorted by mean reward (tree weight); higher is better.}
\label{tab:configs_all}
\end{table}
